# Supplementary material for: Dynamic Spanning Forest with Worst-Case Update Time: Adaptive, Las Vegas, and $O(n^{1/2-\epsilon})$-Time
Source: arXiv:1611.03745 source file (2017-04-17)
Supplement: Supplementary file 1 [file appendix.tex]

\section{Summary of Dynamic $\protect\st$ Algorithms}

\begin{table}[H]
\begin{centering}
\begin{tabular}{|c|c|c|c|c|}
\hline 
Reference & Preprocessing time & Update time & Deterministic? & Against adaptive adversary?\tabularnewline
\hline 
\hline 
\cite{KapronKM13} & $m\polylog n$ & $\log^{5}n$ & Monte Carlo & No\tabularnewline
\hline 
\cite{GibbKKT15} & $m\polylog n$ & $\log^{4}n$ & Monte Carlo & No\tabularnewline
\hline 
\cite{Frederickson85} & $m$ & $\sqrt{m}$ & Yes & Yes\tabularnewline
\hline 
\cite{EppsteinGIN97} & $m$ & $\sqrt{n}$ & Yes & Yes\tabularnewline
\hline 
\cite{Kejlberg-Rasmussen15} & $m$ & $\sqrt{\frac{n(\log\log^{2}n}{\log n}}$ & Yes & Yes\tabularnewline
\hline 
\textbf{This paper} & $m^{1+o(1)}$ & $n^{0.4+o(1)}$ & Monte Carlo & Yes\tabularnewline
\hline 
\textbf{This paper} & $m^{1+o(1)}$ & $n^{0.49305+o(1)}$ & Las Vegas & Yes\tabularnewline
\hline 
\end{tabular}
\par\end{centering}

\caption{Comparison of all known dynamic $\protect\st$ algorithms with worst-case
update time. The term $o(1)=O(\sqrt{\log\log n/\log n})$.}
\end{table}

\begin{table}[H]
\begin{centering}
\begin{tabular}{|c|c|c|c|}
\hline 
Reference & Update time & Deterministic? & Against adaptive adversary?\tabularnewline
\hline 
\hline 
\cite{HenzingerK99} & $\log^{3}n$ & Las Vegas & Yes\tabularnewline
\hline 
\cite{HenzingerT97} & $\log^{2}n$ & Las Vegas & Yes\tabularnewline
\hline 
\cite{HolmLT01} & $\log^{2}n$ & Yes & Yes\tabularnewline
\hline 
\cite{Thorup00} & $\log n(\log\log n)^{3}$ & Las Vegas & Yes\tabularnewline
\hline 
\cite{Wulff-Nilsen13a} & $\log^{2}n/\log\log n$ & Yes & Yes\tabularnewline
\hline 
\cite{HuangHKP-SODA17} & $\log n(\log\log n)^{2}$ & Las Vegas & Yes\tabularnewline
\hline 
\end{tabular}
\par\end{centering}

\caption{Comparison of all known dynamic $\protect\st$ algorithms with amortized
update time. All algorithms assume that the initial graph is empty.}
\end{table}
